# Supplementary material for: Gesture-Aware Zero-Shot Speech Recognition for Patients with Language Disorders
Source: arXiv:2502.13983 source file (2025-02-18)
Supplement: Supplementary file 1 [file appendix.tex]

\section{AphasiaBank Dataset}
As illustrated in Table~\ref{tab:appendix_corpus}, we collected the dataset from the AphasiaBank~\cite{macwhinney2011aphasiabank, forbes2012aphasiabank}, a shared database constructed by experts for aphasia research~\footnote{https://talkbank.org/share/citation.html}.

\begin{table}[h]
\centering
\caption{The corpora from AphasiaBank}
\vspace{-0.1in}
\label{tab:appendix_corpus}
\resizebox{\linewidth}{!}{%
\begin{tabular}{c|c}
\hline
Corpus                                                                & Site                                       \\ \hline \hline
ACWT~\cite{bynek2013aphasiabank}                & Aphasia Center of West Texas               \\
Adler~\cite{adler2013aphasia}                   & Adler Aphasia Center                       \\
APROCSA~\cite{aprocsa2021aphasia}               & Vanderbilt University Medical Center       \\
BU~\cite{bu2013apha}                            & Boston University                          \\
Capilouto~\cite{capilouto2008apha}              & University of Kentucky                     \\
CC-Stark~\cite{cc2022apha}                      & file for CC                                \\
CMU~\cite{cmu2013apha}                          & Carnegie Mellon University                 \\
Elman~\cite{elman2011starting,elman2016aphasia} & Aphasia Center of California               \\
Fridriksson~\cite{Fridriksson2013apha}          & University of South Carolina               \\
Garrett~\cite{Garrett2013apha}                  & Pittsburgh, PA                             \\
Kansas~\cite{kansas2013apha}                    & University of Kansas                       \\
Kempler~\cite{kempler2013apha}                  & Emerson College                            \\
Kurland~\cite{kurland2013apha}                  & University of Massachusetts, Amherst       \\
MSU~\cite{MSU2013apha}                          & Montclair State University                 \\
NEURAL~\cite{neural2023apha}                    & NEURAL Research Lab, Indiana University    \\
Richardson~\cite{Richardson2008apha}            & University of New Mexico                   \\
SCALE~\cite{scale2013apha}                      & Snyder Center for Aphasia Life Enhancement \\
STAR~\cite{star2013apha}                        & Stroke Aphasia Recovery Program            \\
TAP~\cite{tap2013apha}                          & Triangle Aphasia Project                   \\
TCU~\cite{tcu2013apha}                          & Texas Christian University                 \\
Thompson~\cite{thompson2013apha}                & Northwestern University                    \\
Tucson~\cite{tucson2013apha}                    & University of Arizona                      \\
UCL~\cite{ucl2021apha}                          & University College London                  \\
UMD~\cite{faroqi2018comparison}                 & University of Maryland                     \\
UNH~\cite{unh2013apha}                          & University of New Hampshire                \\
Whiteside~\cite{whiteside2013apha}              & University of Central Florida              \\
Williamson~\cite{williamson2013apha}            & Stroke Comeback Center                     \\
Wozniak~\cite{wozniak2013apha}                  & InteRACT                                   \\
Wright~\cite{wright2013apha}                    & Arizona State University                   \\ \hline
\end{tabular}%
}
\end{table}
